# Supplementary material for: Preliminaries paper: Byzantine Tolerant Strong Auditable Atomic Register
Source: arXiv:2309.10664 source file (2023-09-19)
Supplement: Supplementary file 1 [file appendixProof.tex]

% Discussion on the Failure model and auditability proof. For the proof of auditability, we do not let interact Byzantine reader with each other. If we were doing so, obviously, once a Byzantine reader access the data once, it would be impossible to detect the others. However, it is interesting to notice, that even considering an entire cooperative Byzantine behavior, if we could not detect all the Byzantine that access the data, we con detect it at least once. That is, if we consider the $f$ Byzantine servers, and all the Byzantine readers as a unique adversary, then each time the adversary read a new value, our system detect him.
